# Supplementary material for: Can Open Domain Question Answering Systems Answer Visual Knowledge Questions?
Source: arXiv:2202.04306 source file (2022-02-09)
Supplement: Supplementary file 1 [file 7_appendix.tex]

\section{Appendix}

\subsection{Grading Guideline for Human Evaluation}
There are 363 examples to be graded. For each system output, you will have to mark whether the answer and rewritten output given by the system is correct or not (binary). Each example contains an image, a question about the image, a list of gold standard answers from human annotators, and answers from eight Question Answering systems. While evaluating the answers, please keep in mind that for certain questions multiple answers can be possible. Moreover, some of the answers may not appear in the gold standard answer list. So, sometimes you will have to mark correct/incorrect solely based on your judgment. If needed, feel free to look up the question on the internet. Certain questions require the answers to be ``numbers" (such as calorie content in food or year of invention of a certain machine). You can mark the answer correct if the predicted answers is around the same timeline as the gold answers (e.g., 19th century for 1890). 

%While evaluating the rewrites, we need to make sure that the correct span (e.g., ``this animal") is substituted by the correct entity (e.g, ``the giraffe"). Please keep in mind that the rewrite does not have to completely grammatically. For example, if we solely replace ``this" in this case and rewrite to ``how tall is giraffe animal", it still makes sense to human beings and has sufficient information for the text-based QA model to generate good answer, so we want to mark this kind of rewrite as correct as well. 
